# Supplementary material for: AlphaMatch: Improving Consistency for Semi-supervised Learning with Alpha-divergence
Source: arXiv:2011.11779 source file (2020-11-23)
Supplement: Supplementary file 1 [file appendix.tex]

\section{Proof of Optimal $\gamma(\cdot|x)$ in Eq~\ref{equ:gammat}}
\begin{proof}
Consider optimization of form  
$$
\min_{\gamma } \sum_{i} w_i [D_\alpha(\gamma ~||~p_i) ] = 
\sum_i w_i (\int \frac{\gamma^\alpha}{p_i^{\alpha-1}}-1). 
$$ %yields that 
We have 
$$
\gamma \propto  
\left  (\sum_i w_i p_{i}^{\red{1-\alpha}}\right )^{\frac{1}{\red{1- \alpha}}}
$$

\begin{align*}
\sum_i w_i \sum_x \frac{\gamma^\alpha(x)}{p_i^{\alpha-1}(x)} 
&= \sum_x \sum_i w_i p_i^{1-\alpha} (x) \gamma^\alpha(x),  \\
&= \sum_x \bar{p}^{1-\alpha}(x) \gamma^\alpha(x), ~~\text{where} ~\bar{p}(x) = \bigg(\sum_i w_i p_i^{1-\alpha}(x)\bigg)^{\frac{1}{1-\alpha}} \\ 
&= D_\alpha(\gamma || z \bar{p}), 
\end{align*}
where $z$ is the normalization constant, therefore, we have
$\gamma^* \propto \bar{p}$.
\end{proof}
